# Supplementary material for: First- and Second-Order Bounds for Adversarial Linear Contextual Bandits
Source: arXiv:2305.00832 source file (2023-05-24)
Supplement: Supplementary file 1 [file appendixD.tex]

\section{Proof of Theorem 2}
Let decompose our estimate $\ttheta_{t,a} = \htheta_{t,a}^* + b_{t,a}$, where $\EEt{\htheta_{t,a}^*} = \theta_{t,a}$. We can directly get the following bound from Lemma~\ref{ghost}:
\begin{align}\label{regret_bias}
	\sum_{t=1}^T\EEt{  \iprod{Z_t(X_t) -  Z^*(X_t)}{\theta_t}  } = 	\sum_{t=1}^T \EEt{   \iprod{Z_t(X_0) -  Z^*(X_0)}{\ttheta_t}} + 2 \sum_{t=1}^T \max_a |\EE{ \siprod{X_t}{b_{t,a}}}|.
\end{align}

Following useful properties of matrix geometric resampling from Lemma~D.1 in \cite{LWL21}:
\begin{lemma}
	Let $\varepsilon > 0 $ and define $M = \lceil \frac{24 \ln(dHT)}{\epsilon^2}\frac{4}{\lambda^2 \ln^2\frac{1}{\varepsilon \lambda}}\rceil $ and $N = \lceil \frac{2}{\lambda}\ln \frac{1}{\varepsilon \lambda} \rceil$. Let $\mathcal{T}$ be a set of $MN$ trajectories generated by $\pi$. Then, Geometric resampling with input $\pa{\mathcal{T}, M, N }$ ensures the following:
	\begin{align}\label{cov_norm1}
		\norm{\hSp_{t}}_{op} \le  \frac{2}{\lambda} \ln \frac{1}{\varepsilon \lambda},
	\end{align} 
	\begin{align}\label{cov_norm2}
	\norm{\EE{\hSp_{t} } - \Sigma_t^{-1} }_{op} \le \epsilon,
	\end{align} 
	\begin{align}\label{cov_norm3}
	\norm{\hSp_{t}  - \Sigma_t^{-1} }_{op} \le \epsilon,
	\end{align} 
	\begin{align}\label{cov_norm4}
	\norm{\hSp_{t}  \Sigma_t }_{op} \le 1+ 2\epsilon,
	\end{align} 
where (\ref{cov_norm3}) and  (\ref{cov_norm4}) hold with probability at least $1-1/T^3$. 
\end{lemma}
\begin{proof}
	For (\ref{cov_norm1}), notice that each of $\hSpm_{t}$, $m=1,\dots, M$ is a sum of $N+1$ terms.  The $n-$th term of them  has an operator norm upper bounded by $c$.
	\begin{align*}
		\norm{\hSpm_{t}}_{op} \le \sum_{n=0}^{N_t} c(1-c\gamma)^n \le c(N_t+1)\le  \frac{2}{\lambda_t} \ln \frac{1}{\varepsilon \lambda_t}, 
	\end{align*}
by the definition of $N$ and $c = 1/2$. As $\hSp_{t}$ is an average of $\hSpm_{t}$, this implies (\ref{cov_norm1}).
To show (\ref{cov_norm2}), notice that $\EEt{Y_n} = \Sigma_t$ and $\{ Y_n\}^N_{n=1}$ are independent. We get
\begin{align*}
	\EEt{\hSp_{t}} = \EE{\hSpm_{t}} = cI + c\sum_{i=1}^N\pa{I - c \Sigma_t}^i = \Sigma_t^{-1}\pa{I - \pa{I - c \Sigma_t}^{N+1} },
\end{align*}
where in  the last step we used that $I + \sum_{i=1}^N A^i = (I - A)^{-1}(I - A^{N+1})$ with $A = I - c\Sigma_t$. Thus,
\begin{align*}
	\norm{ \EEt{\hSp_{t}}  - \Sigma_t^{-1}}_{op} = \norm{ \Sigma_t^{-1} \pa{ I - c \Sigma_t }^{N+1} }_{op} \le \frac{ \exp\pa{- c\lambda_{\min}(\Sigma_t)(N+1)} }{\lambda_{min}(\Sigma_t)} \le T^2 \frac{ \exp\pa{- c\lambda_{\min} \frac{N+1}{T^2}} }{\lambda_{min}}
\end{align*}
\end{proof}

From (\ref{regret_bias}) and Lemma~\ref{exp3proof_adaptive} with $\Omega =  \{w \in \Delta^K: w_{a} \ge \frac{1}{T}, \forall a \in[K]\}$ and $m_t = \bar 0$, we get for the second term of (\ref{regret_dec}):

\begin{align}\label{expectation_decomp_2}
	&\EE{ \sum_{t=1}^T \iprod{Z_t(X_t) -  Z^*(X_t)}{\theta_t}  } = \EE{  \sum_{t=1}^T \iprod{Z_t(X_0) -  Z^*(X_0)}{\ttheta_t}}  +  2 \sum_{t=1}^T \max_a |\EE{ \siprod{X_t}{b_{t,a}}}| \nonumber \\
	&\qquad \le \EE{ \sum_{t=1}^T     \frac{1}{\eta_t}     \psi( -\eta_t \iprod{Z_t(X_0)}{\ttheta_t} )
		+ \frac{1}{T}\sum_{t=1}^T  \iprod{ z(q_0 - \pi^*(X_0) , X_0) }{\ttheta_t} + \frac{K \log T}{\eta_T} } +  2 \sum_{t=1}^T \max_a |\EE{ \siprod{X_t}{b_{t,a}}}|.
\end{align} 

Bound on the bias of the estimator:
\begin{lemma}
	$bias_t = \EEt{ \siprod{Z_t(X_t)}{\theta_{t,a}  - \ttheta_{t,a}}} - \EEt{ \siprod{z(, \pi^*(X_t))}{\theta_{t,a}  - \ttheta_{t,a}}} \le d\varepsilon.$
\end{lemma}
\begin{proof}	
	\begin{align*}
		bias_t &= \EEt{ \siprod{Z_t(X_0)}{\theta_{t,a}  - \ttheta_{t,a}}} - \EEt{ \siprod{z(X_0, \pi^*(X_0))}{\theta_{t,a}  - \ttheta_{t,a}}} \\
		& =  \EE{ X_t\transpose \pa{\Sigma^{-1}_{t,a} - \hSp_{t,a}}X_t X_t\transpose\theta_{t,a} \II{A_t = a} } 
	\end{align*}
	Using (\ref{cov_norm2}), we get 
	\begin{align*}
		\EEt{ \siprod{X_t}{\theta_{t,a}  - \ttheta_{t,a}}} &= \EE{ X_t\transpose \pa{\Sigma^{-1}_{t,a} - \hSp_{t,a}}X_t X_t\transpose\theta_{t,a} \II{A_t = a} } \le \trace{\Sigma \pa{ \Sigma^{-1}_{t,a} - \EEt{\hSp_{t,a} }}} \le d \norm{ \Sigma }_{op} \norm{ \Sigma^{-1}_{t,a} - \EEt{\hSp_{t,a} }}_{op}\\
		\le d\varepsilon 
	\end{align*}
\end{proof}

For the first term in (\ref{expectation_decomp_2}), we show the following:

\begin{lemma}\label{quadratic_unknown}
	$\EEt{\psi(-\eta_t \iprod{Z_t(X_0)}{\ttheta_t})} \le 2\eta_t^2  d^2K^2 \EEt{  \ell_t(A_t, X_t)}    + \tOO\pa{\frac{d^2K^2 }{T}} 	$.
\end{lemma}
\begin{proof}
	We first show the following property: $\EEw{\eta_t^2 \iprod{Z_t(X_0)}{\ttheta_t}^2}{Z_t(X_0)} \le \frac{1}{100}$:
	\begin{align*}
		\EEw{\eta_t^2 \iprod{Z_t(X_0)}{\ttheta_t}^2}{Z_t(X_0)} &\le \EEw{\eta_t^2 \trace{\Sigma_t \hSp_{t}} Z_t(X_t)\transpose  \hSp_{t}  Z_t(X_t) }{Z_t(X_0)} \le \eta_t^2 d\sigma^2 \frac{4}{\lambda^2}\ln^2 \frac{1}{\varepsilon \lambda} \le  \frac{1}{100}.
	\end{align*}\todo{tune $\eta_t$ accordingly.}
Then, by Lemma 6 of \cite{NEURIPS2020_15bb63b2}, we have:
\begin{equation*}
	\EEt{\psi(-\eta_t \iprod{Z_t(X_0)}{\ttheta_t})} \le 2\eta_t^2 \EEt{\iprod{Z_t(X_0)}{\ttheta_t}^2}.
\end{equation*}
We now show:
	\begin{align}
	\EEt{\iprod{Z_t(X_0)}{\ttheta_t}^2 } &\le	\EEt{ \eta_t^2 \ell_t(A_t, X_t) \trace{ \hSp_{t} Z_t(X_0)Z_t(X_0)\transpose \hSp_{t} Z_t(X_t)Z_t(X_t)\transpose   }} \nonumber \\
	& = \eta_t^2	\EEt{  \ell_t(A_t, X_t) \trace{ \hSp_{t} \Sigma_t \hSp_{t} Z_t(X_t)Z_t(X_t)\transpose   }} \nonumber\\
	& = \eta_t^2	\EEt{  \ell_t(A_t, X_t) \trace{ \pa{\hSp_{t}}^{1/2^T} \Sigma_t  \pa{\hSp_{t}}^{1/2} }\trace{ Z_t(X_t) \transpose  \hSp_{t} Z_t(X_t) } } \nonumber\\
	& = \eta_t^2	\EEt{  \ell_t(A_t, X_t) \trace{ \hSp_{t} \Sigma_t  }\trace{ Z_t(X_t)\transpose  \hSp_{t} Z_t(X_t) } } 
\end{align}
We make use of  Lemma~D.1 in \cite{LWL21}, we get from (28) $\norm{\hSp_{t}}_{op} \le  \frac{2}{\lambda} \ln \frac{1}{\varepsilon \lambda} $ from (31) we get that with probability at least $1- \frac{1}{T^3}$,  $\norm{\hSp_{t} \Sigma_t }_{op} \le 1 + \varepsilon$. Define event $H_t = \bigg\{ \norm{\hSp_{t} \Sigma_t }_{op} \le 1 + \varepsilon  \bigg\}$, then 
\begin{align*}
	&\EEt{  \ell_t(A_t, X_t) \trace{ \hSp_{t} \Sigma_t  }\trace{ Z_t(X_t) \hSp_{t} Z_t(X_t)\transpose  } }\\
	&\qquad \le 	\EEt{  \ell_t(A_t, X_t) (1+\epsilon) dK\trace{ Z_t(X_t) \hSp_{t} Z_t(X_t)\transpose  } \II{H_t}} + 	\EEt{  \ell_t(A_t, X_t) \trace{ \hSp_{t} \Sigma_t  } \trace{ Z_t(X_t)\transpose  \hSp_{t} Z_t(X_t)  } \II{\overline H_t}}\\
	&\qquad \le 	\EEt{  \ell_t(A_t, X_t) (1+\epsilon) dK\trace{ Z_t(X_t)\transpose \pa{ \Sigma_t^{-1} - \pa{I-\beta \Sigma_t}^M} Z_t(X_t)  } } + 	\frac{1}{T^3} d^2K^2  \frac{2}{\lambda} \ln \frac{1}{\varepsilon \lambda} \\
	&\qquad \le 	\EEt{  \ell_t(A_t, X_t) (1+\epsilon) dK\trace{ Z_t(X_t)\transpose  \Sigma_t^{-1}   Z_t(X_t) } } + 	\frac{1}{T^3} d^2K^2 \sigma^4  \frac{2}{\lambda} \ln \frac{1}{\varepsilon \lambda}  . 
\end{align*}
Define event $\mathcal{G}_t = \{Z_t(X_t)\transpose  \Sigma_t  Z_t(X_t) \le \frac{1}{T} \}$. Then,
\begin{align*}
	&\EEt{  \ell_t(A_t, X_t) (1+\epsilon) dK\trace{ Z_t(X_t)\transpose  \Sigma_t^{-1}   Z_t(X_t) } } + 	\frac{1}{T^3} d^2K^2 \sigma^4  \frac{2}{\lambda} \ln \frac{1}{\varepsilon \lambda} \\
	&\quad\le \EEt{  \ell_t(A_t, X_t) (1+\epsilon) dK\pa{dK\sigma^2\II{\mathcal{G}_t } + \sigma^2 dK \II{ \overline{\mathcal{G}}_t } }} + 	\frac{1}{T^3} d^2K^2  \frac{2}{\lambda} \ln \frac{1}{\varepsilon \lambda}  \\
	&\quad\le \EEt{  \ell_t(A_t, X_t)} (1+\epsilon) d^2K^2 + dK\frac{1}{T}   + 	\frac{1}{T^3} d^2K^2  \frac{2}{\lambda} \ln \frac{1}{\varepsilon \lambda}. \\
\end{align*}
Collecting all terms together, we get a statement of the lemma. 
\end{proof}

\begin{align*}
	R_T &\le \EE{\sum_{t=1}^T \frac{1}{\eta_t} \psi(-\eta_t \iprod{Z_t(X_0)}{\ttheta_t}) } +  \EE{ \frac{K \log T}{\eta_T}} + 2 d\epsilon T +  2. 
\end{align*}
By Lemma~\ref{quadratic_unknown}:
\begin{align*}
	&\EE{\sum_{t=1}^T \frac{1}{\eta_t} \psi(-\eta_t \iprod{Z_t(X_0)}{\ttheta_t}) } \le \EE{\sum_{t=1}^T 2\eta_t  d^2K^2  \ell_t(A_t, X_t)   + \tOO\pa{\frac{d^2K^2 }{T}} }  =   2 d^2K^2\EE{\sum_{t=1}^T \eta_t   \ell_t(A_t, X_t) }  + \tOO\pa{d^2K^2},   
\end{align*}
 Let $\mathcal{E}_T$ be an event that for all $t\in[1,T]$, (\ref{concentration_ineq_right}) with $\delta = 1/T$.  From Lemma~\ref{freedman_coef}, we get:
 \begin{align*}
 	&\EE{\sum_{t=1}^T \eta_t \ell_t(A_t, X_t) } = \EE{ \sum_{t=1}^T \eta_t\ell_t(A_t, X_t)\II{\mathcal{E}_T}} + \EE{ \sum_{t=1}^T \eta_t\ell_t(A_t, X_t)\II{\overline{\mathcal{E}}_T}}\\
 	&\le \frac{1}{10 \sqrt{2dK}} \sum_{t=1}^T \frac{L_t - L_{t-1}}{\sqrt{L_t}}  + \frac{1}{T} \sqrt{K}  T 
 	\\
 	&= \frac{1}{10 \sqrt{2dK}} \sum_{t=1}^T \frac{(\sqrt{L_t} - \sqrt{L_{t-1}})(\sqrt{L_t} + \sqrt{L_{t-1}})}{\sqrt{L_t}}    + \sqrt{K}\\
 	&\le \frac{2}{10 \sqrt{2dK}} \sum_{t=1}^T (\sqrt{L_t} - \sqrt{L_{t-1}})   +   \sqrt{K}\\
 	&\le \frac{2}{10 \sqrt{2dK}} \sqrt{L_T} + \sqrt{K}, 
 \end{align*}

where $\eta_t = \frac{1}{10}\pa{2dK\pa{\hL_t+1 + G_t}}^{-1/2}$, $\lambda_t = \pa{\hL_t+1}^{-1/2}$.
\todo{express through $L_T^*$}
