# Supplementary material for: First- and Second-Order Bounds for Adversarial Linear Contextual Bandits
Source: arXiv:2305.00832 source file (2023-05-24)
Supplement: Supplementary file 2 [file appendixE.tex]

\section{Computation of Z}
Since we have one redundant degree of freedom and
\begin{equation*}
\sum_{a=1}^{K}q_{a}\iprod{\varphi(x,a)}{\hat{\Theta}_{t-1}} = \sum_{a=1}^{K-1}q_{a}\iprod{\varphi(x,a)-\varphi(x,K)}{\hat{\Theta}_{t-1}}+ \iprod{\varphi(x,K)}{\hat{\Theta}_{t-1}}
\end{equation*}
$p(q|x)$ may be rewritten as 
\begin{align*}
p(q|x)&= \frac{e^{-\eta\sum_{a=1}^{K}q_{a}\iprod{\varphi(x,a)}{\hat{\Theta}_{t-1}}}}{\int_{\sum_{a=1}^{K-1}q'_{a} \leq 1}e^{-\eta\sum_{a=1}^{K}q'_{a}\iprod{\varphi(x,a)}{\hat{\Theta}_{t-1}}}\mathrm{d}q'} \\
&= \frac{\prod_{a=1}^{K-1}e^{\eta q_{a}\iprod{\varphi(x,K)-\varphi(x,a)}{\hat{\Theta}_{t-1}}}}{\int_{\sum_{a=1}^{K-1}q'_{a} \leq 1} e^{\eta q'\iprod{\varphi(x,K)-\varphi(x,a)}{\hat{\Theta}_{t-1}}}\mathrm{d}q'}.
\end{align*}
W.l.o.g. permute the arms such that the redundant degree of freedom $K$ is that with the smallest estimated loss, thus defining $c_{a}-c_{K}=\iprod{\varphi(x,a)-\varphi(x,K)}{\hat{\Theta}_{t-1}} \geq 0$ we have that
\begin{equation}\label{sampling_dist}
p(q|x)=\frac{\prod_{a=1}^{K-1}e^{- (c_{a}-c_{K})q_{a}}}{Z}\mathbb{I}_{\left\{\sum_{a=1}^{K-1}q_{a}\leq 1\right\}}
\end{equation}
where $Z=\int_{\sum_{a=1}^{K-1}q'_{a} \leq 1} e^{-\iprod{q'}{c}}\mathrm{d}q'$.

\begin{lemma}\label{intcalc}
Let $K'\leq K$ and $a'$ denote a relabelling of the arms $a\in[K]$ such that $c_{1}>\dots>c_{K'}$ and $c_{i},c_{j}\rightarrow c_{i'}$ if $c_{i}=c_{j}$. Then normalization constant $Z=e^{c_{K}}\int_{\Delta_{K}}e^{-\iprod{q}{c}}\mathrm{d}q$ admits the following representation
\begin{equation*}
Z=\sum_{a'=1}^{K'}\left(b_{a'1}+ \dots +\frac{b_{a'd_{a'}}}{\Gamma(d_{a'})}\right)e^{-(c_{a'}-c_{K})},
\end{equation*}
where $d_{a'}\in[K]$ denotes the multiplicity of the coefficient $c_{a'}$ and the coefficients $b_{ij}$ can be computed in $O\left(K\mathrm{log}^{2}K\right)$ computational steps.
\end{lemma}
\begin{proof}
The proof is an instantiation of \cite{blog}. Note that the integral may be written
\begin{align}
\label{convolve1}
\begin{split}
\int_{\Delta_{K}}e^{-\iprod{q}{c}}\mathrm{d}q &= \int_{0}^{1}\int_{0}^{1-q_{1}}\dots \int_{0}^{1-\sum_{a}^{K-2}q_{a}} e^{-c_{K}(1-\sum_{a=1}^{K-1}q_{a})}\prod_{a=1}^{K-1}e^{-c_{a}q_{a}}\mathrm{d}q_{K-1}\dots\mathrm{d}q_{1} \\
&=\int_{0}^{\zeta_{0}}\int_{0}^{\zeta_{1}}\dots \int_{0}^{\zeta_{K-2}} e^{-c_{K}(\zeta_{K-2}-q_{K-1})}\prod_{a=1}^{K-1}e^{-c_{a}q_{a}}\mathrm{d}q_{K-1}\dots\mathrm{d}q_{1}
\end{split}
\end{align}
where we have defined $\zeta_{k}=1-\sum_{1}^{K-k}\zeta_{a}$ for convenience. The inner integral over $q_{K-1}$ is simply a convolution
\begin{equation*}
\int_{0}^{\zeta_{K-2}} e^{-c_{K}(\zeta_{K-2}-q_{K-1})}e^{-c_{K-1}q_{K-1}}\mathrm{d}q_{K-1} = (e^{-c_{K-1}q} \star e^{-c_{K}q})(\zeta_{K-2}),
\end{equation*}
leaving the integral to be written as 
\begin{equation}
\label{convolve2}
\int_{0}^{\zeta_{0}}\int_{0}^{\zeta_{1}}\dots \int_{0}^{\zeta_{K-3}} (e^{-c_{K-1}q} \star e^{-c_{K}q})(\zeta_{K-3}-q_{K-2})\prod_{a=1}^{K-2}e^{-c_{a}q_{a}}\mathrm{d}q_{K-2}\dots\mathrm{d}q_{1},
\end{equation}
where in the argument of the convolution we have made use of the fact that $\zeta_{K-2}=\zeta_{K-3}-q_{K-2}$. Now the integral (\ref{convolve2}) is of the same form as the last line of (\ref{convolve1}), and the process can be repeated with successive ordered convolutions, leaving the final result of this process as
\begin{equation*}
\int_{\Delta_{K}}e^{-\iprod{q}{c}}\mathrm{d}q = (e^{-c_{1}q} \star \dots \star e^{-c_{K}q})(\zeta_{0}).
\end{equation*}
Let $\mathcal{L}[f](s)=\mathcal{F}(s)=\int_{0}^{\infty}e^{-st}f(t)\mathrm{d}t$ be the Laplace transform of a function $f:\reals \rightarrow \reals$ and $\mathcal{L}^{-1}$ be its inverse, then applying the convolution theorem gives
\begin{equation*}
(e^{-c_{1}q} \star \dots \star e^{-c_{K}q})(\zeta_{0})=\mathcal{L}^{-1}\left[\mathcal{L}\left[(e^{-c_{1}q} \star \dots \star e^{-c_{K}q})\right]\right](\zeta_{0})= \mathcal{L}^{-1}\left[\prod_{a=1}^{K}\frac{1}{s+c_{a}}\right](\zeta_{0}).
\end{equation*}
Now consider the partial fraction, and order the indices s.t. $c_{1} > \dots > c_{K'}$, where $K'\leq K$ and equal values are given the same index, then the argument of $\mathcal{L}^{-1}$ becomes;
\begin{align*}
\prod_{a=1}^{K}\frac{1}{s+c_{a}} &= \prod_{a'=1}^{K'}\frac{1}{(s+c_{a'})^{d_{a'}}} \\
&= \sum_{a'=1}^{K'}\left(\frac{b_{a'1}}{s+c_{a'}}+ \dots +\frac{b_{a'd_{a'}}}{(s+c_{a'})^{d_{a'}}}\right),
\end{align*}
where $b_{ij}$ are coefficients which may be calculated via e.g. via the method of residues or a partial fraction decomposition, which requires $O(K\mathrm{log}^{2}K)$ steps of computation in total \cite{kung}. By linearity of $\mathcal{L}^{-1}$ and using $\mathcal{L}^{-1}\left[\frac{1}{(s+a)^{n}}\right](t)=\frac{t^{n-1}e^{-at}}{\Gamma(n)}$, we're left with
\begin{align*}
\int_{\Delta_{K}}e^{-\iprod{q}{c}}\mathrm{d}q&=\sum_{a'=1}^{K'}\left(b_{a'1}e^{-c_{a'}\zeta_{0}}+ \dots +\frac{b_{a'd_{a'}}\zeta_{0}^{d_{a'}-1}e^{-c_{a'}\zeta_{0}}}{\Gamma(d_{a'})}\right) \\
&=\sum_{a'=1}^{K'}\left(b_{a'1}+ \dots +\frac{b_{a'd_{a'}}}{\Gamma(d_{a'})}\right)e^{-c_{a'}}.
\end{align*}
\end{proof}
